# Supplementary material for: Sharpened Lazy Incremental Quasi-Newton Method
Source: arXiv:2305.17283 source file (2024-03-12)
Supplement: Supplementary file 1 [file generalized_sharpened_iqn.tex]

\input{broyden_class_extension}
